# Supplementary material for: A Two-Stage Approach for Segmenting Spatial Point Patterns Applied to Multiplex Imaging
Source: arXiv:2412.08828 ancillary file (2024-12-12)
Supplement: Supplementary file 1 [file updated_supplementary_materials.pdf]

# A Two-Stage Approach for Segmenting Spatial Point Patterns Applied to Multiplex Imaging Supplementary Materials

**Alvin Sheng[1,*], Brian J Reich[2], Ana-Maria Staicu[2], Santhoshi N Krishnan[4,5], Arvind Rao[3,4,5,7,8],**

**and**

**Timothy L Frankel[6]**

[1]Division of Biostatistics and Health Data Science, University of Minnesota, Minneapolis, MN, USA

[2]Department of Statistics, North Carolina State University, Raleigh, NC, USA

[3]Department of Biostatistics, University of Michigan, Ann Arbor, MI, USA

[4]Department of Computational Medicine and Bioinformatics, University of Michigan, Ann Arbor, MI, USA

[5]Department of Electrical and Computer Engineering, Rice University, Houston, TX, USA

[6]Department of Surgery, University of Michigan, Ann Arbor, MI, USA

[7]Department of Radiation Oncology, University of Michigan, Ann Arbor, MI, USA

[8]Department of Biomedical Engineering, University of Michigan, Ann Arbor, MI, USA

**email:* sheng123@umn.edu

## 1. Web Appendix A: First- and second-order characteristics of SPPs

The stochastic behavior of an SPP can be described by its first- and second-order characteristics. Denote by the real-valued function $L_{nh}(B)$ the count of cells with type $h$ in subregion $B \subset W_n$. The random quantity $L_{nh}(\cdot)$ can be characterized through the intensity function $\lambda_{nh}(\mathbf{s}) \geqslant 0$:

$$E\{L_{nh}(B)\} = \int_B \lambda_{nh}(\mathbf{s}) d\mathbf{s} \tag{S1}$$

The intensity function is a first-order characteristic. Similarly, by ignoring the cell types, denote by $L_n(B)$ the total count of cells in subregion $B$ and let $\lambda_n(\cdot)$ be the marginal intensity function corresponding to $L_n(\cdot)$, defined as $\lambda_n(\mathbf{s}) = \sum_{h=1}^{H} \lambda_{nh}(\mathbf{s})$.

The product density function $\lambda_n^{(2)}(\mathbf{s}, \mathbf{s}')$ is a second-order characteristic that quantifies the dependence between spatial locations. It is analogous to the covariance of two random variables. We define it similarly to the intensity function: let $B_1, B_2 \subset W_n$ be two random subregions of $W_n$. Then, the expected number of pairs of cells $E[L_n(B_1)L_n(B_2)]$ is determined by $\lambda_n^{(2)}(\mathbf{s}, \mathbf{s}') \geqslant 0$, i.e.,

$$E\{L_n(B_1)L_n(B_2)\} = \int_{B_1} \int_{B_2} \lambda_n^{(2)}(\mathbf{s}, \mathbf{s}') d\mathbf{s} d\mathbf{s}'. \tag{S2}$$

If the spatial locations $\mathbf{s}$ and $\mathbf{s}'$ are sampled independently, then $\lambda_n^{(2)}(\mathbf{s}, \mathbf{s}') = \lambda_n(\mathbf{s})\lambda_n(\mathbf{s}')$. Note that it is also possible to allow for the second-order characteristic to vary by cell type, but due to the large number of cell types in our application, we assume the same second-order dependence regardless of cell type.

The quantity that combines the product density function and the marginal intensity is the pair correlation function (PCF), denoted as $g_n$. It is a second-order characteristic that measures the interaction between spatial locations, and is defined as

$$g_n(\mathbf{s}, \mathbf{s}') = \frac{\lambda_n^{(2)}(\mathbf{s}, \mathbf{s}')}{\lambda_n(\mathbf{s})\lambda_n(\mathbf{s}')}. \tag{S3}$$

If there is independence between points $\mathbf{s}$ and $\mathbf{s}'$ (in the case of complete spatial randomness), then $g_n(\mathbf{s}, \mathbf{s}') = 1$. If the points tend to attract each other, then $g_n(\mathbf{s}, \mathbf{s}') > 1$; if the points tend to repel each other, then $g_n(\mathbf{s}, \mathbf{s}') < 1$. Although $g_n$ has a similar interpretation to the correlation, its range is in fact $[0, \infty)$ and not $[-1, 1]$.

## 2. Web Appendix B: Additional computational details

### 2.1 *Web Appendix B.1: Metropolis within Gibbs Sampling*

To conduct inference with the PCM, we implement MCMC sampling in R (R Core Team, 2021) to approximate the posterior distribution of the cluster labels and regime-specific parameters. Specifically, we implement the Metropolis within Gibbs algorithm (Chib and Greenberg, 1995).

Gibbs updates are used for $\mu_{q\eta}$, $C_{nl}$, and $\nu_q^2$, which have conjugate priors (see Section 2.2 and Equation 19 in the main article). The full conditional for $\mu_{q\cdot}, q = 1, \ldots, Q$ is

$$\begin{aligned}
\mu_{q\cdot}|\cdot &\sim MVN(VU, V) \\
V &= \left(\frac{1}{\nu_q^2}\sum_{n=1}^{N}\mathcal{C}_n^{\intercal}\mathcal{C}_n + I_M\right)^{-1} \\
U &= \frac{1}{\nu_q^2}\sum_{n=1}^{N}\mathcal{C}_n^{\intercal}\hat{\xi}_{n\cdot q} \\
\mathcal{C}_n &= \begin{bmatrix} \mathbf{I}(C_{n1} = 1) & \cdots & \mathbf{I}(C_{n1} = M) \\ \vdots & & \vdots \\ \mathbf{I}(C_{nL} = 1) & \cdots & \mathbf{I}(C_{nL} = M) \end{bmatrix}.
\end{aligned} \tag{S4}$$

The full conditional for $C_{nl}, n = 1, \ldots, N, l = 1, \ldots, L$ is

$$p(C_{nl}=\eta|\cdot) \propto \exp\left\{\alpha_\eta + \psi \sum_{l' \in \mathcal{N}_{nl}} \mathbf{I}(C_{nl'}=\eta)\right\} \exp\left\{-\frac{1}{2}\sum_{q=1}^{Q}\frac{1}{\nu_q^2}(\hat{\xi}_{nlq}-\mu_{q\eta})^2\right\}, \quad \text{(S5)}$$

where $\mathcal{N}_{nl}$ is the set of indices $l'$ such that grid region $W_{nk}$ is adjacent to grid region $W_{nl}$. Finally, the full conditional for $\nu_q^2$, $q = 1, \ldots, Q$ is

$$\nu_q^2|\cdot \sim InvGamma\left(\frac{NL}{2}+1, \frac{1}{2}\sum_{n=1}^{N}(\hat{\xi}_{n\cdot q}-\mathcal{C}_n\mu_{q\cdot})^\intercal(\hat{\xi}_{n\cdot q}-\mathcal{C}_n\mu_{q\cdot})+0.01\right). \quad \text{(S6)}$$

On the other hand, Metropolis-Hastings sampling is used for $\psi$ and $\alpha_\eta$. All Metropolis-Hastings updates use truncated normal candidate distributions. The candidate distributions were tuned during the burn-in phase to have acceptance rates between 0.3 and 0.5. Simulated annealing was used during the burn-in phase to encourage more exploration of the parameter space at the beginning of burn-in (Reich and Ghosh, 2019). Convergence is monitored using traceplots and effective sample sizes for several representative parameters.

2.1.1 *Web Appendix B.1.1: Evaluating the normalizing constant for the spatial Potts model.* The Metropolis-Hastings updates for the spatial Potts parameters involve the major computational challenge of evaluating the normalizing constant $d(\boldsymbol{\theta})$ (Equation 11 in the main article). Because the normalizing constant does not depend on the subject index $n$, and $\alpha_1$ has been set to 0, we drop $n$ and $\alpha_1$ in the below exposition for ease of notation. To estimate $d(\boldsymbol{\theta})$, we adapt a computational method suggested by Reich and Gardner (2014). The method is based on the identity

$$\frac{\partial}{\partial\psi}\log\{d(\psi,\alpha_2,\ldots,\alpha_M)\} = E\left\{\sum_{l\sim l'}\mathbf{I}(C_l=C_{l'})\middle|\psi,\alpha_2,\ldots,\alpha_M\right\}, \quad \text{(S7)}$$

where the expectation is with respect to the spatial Potts model for $C_1, \ldots, C_L$ with parameters $\psi, \alpha_2, \ldots, \alpha_M$. The identity is a property of exponential families; see Equation 3.4.4 in

Theorem 3.4.2 of Casella and Berger (2002). Because $\log\{d(\boldsymbol{\theta})\}$ is an antiderivative of the expectation in terms of $\psi$, we have

$$\int_0^{\psi} E\left\{\sum_{l\sim l'} \mathbf{I}(C_l = C_{l'}) \middle| \psi', \alpha_2, \ldots, \alpha_M\right\} d\psi' = \log\{d(\psi, \alpha_2, \ldots, \alpha_M)\} - \log\{d(0, \alpha_2, \ldots, \alpha_M)\} \tag{S8}$$

Likewise, for $\alpha_\eta$ we have the identity

$$\frac{\partial}{\partial \alpha_\eta} \log\{d(\psi, \alpha_2, \ldots, \alpha_M)\} = E\left\{\sum_{l=1}^{L} \mathbf{I}(C_l = \eta) \middle| \psi, \alpha_2, \ldots, \alpha_M\right\}, \tag{S9}$$

where the expectation is with respect to the spatial Potts model for $C_1, \ldots, C_L$ with the given parameters. Because $\log\{d(\boldsymbol{\theta})\}$ is an antiderivative of the expectation in terms of $\alpha_\eta$, we have

$$\int_0^{\alpha_\eta} E\left\{\sum_{l=1}^{L} \mathbf{I}(C_l = \eta) \middle| \psi, \alpha_2, \ldots, \alpha_\eta, \ldots, \alpha_M\right\} d\alpha'_\eta = \\ \log\{d(\psi, \alpha_2, \ldots, \alpha_\eta, \ldots, \alpha_M)\} - \log\{d(\psi, \alpha_2, \ldots, 0, \ldots, \alpha_M)\} \tag{S10}$$

for $\eta = 2, \ldots, M$. Approximating the integral of the expectations in (S8) and (S10) will provide us with the quantities needed in the Metropolis-Hastings updates for $\psi$ and $\alpha_\eta$.

Let $\mathbf{T} = \left(\sum_{l\sim l'} \mathbf{I}(C_l = C_{l'}), \sum_{l=1}^{L} \mathbf{I}(C_l = 2), \ldots, \sum_{l=1}^{L} \mathbf{I}(C_l = M)\right)$ be the vector of sufficient quantities for which we need the expectations. We seek to estimate the expectation of $\mathbf{T}$ with respect to the spatial Potts model for selected values of $\boldsymbol{\theta} = (\psi, \alpha_2, \ldots, \alpha_M)$ within the domain $[0, 2.5] \times [-5, 5]^{M-1}$ (see Section 2.2 in the main article for a discussion of the selected bounds). We focus on the grid of $\psi$ values $0, 0.01, \ldots, 2.5$; for each $\psi$ value, we randomly generate 100,000 $(\alpha_2, \ldots, \alpha_M)$ vectors from a truncated multivariate normal distribution with mean $\mathbf{0}$, covariance matrix $\text{diag}(16, \ldots, 16)$, and truncated support $[-5, 5]^{M-1}$.

For a given $\boldsymbol{\theta}$, we generate 100 realizations of the spatial Potts model and calculate the

average of $\mathbf{T}$ across realizations. The realizations were generated using MCMC methods in the R package `potts` (Geyer and Johnson, 2022). A burn-in of 200 MCMC iterations was used for each realization, and the previous draw was used as the initial value for the subsequent realization. This results in the estimate $\hat{E}(\mathbf{T}|\boldsymbol{\theta}) = \frac{1}{100}\sum_{i=1}^{100}\mathbf{T}_i$.

After estimating $\hat{E}(\mathbf{T}|\boldsymbol{\theta})$ for all selected $\boldsymbol{\theta}$, we interpolate over the $\hat{E}(\mathbf{T}|\boldsymbol{\theta})$ values with a gradient boosted trees model, implemented via the eXtreme Gradient Boosting algorithm (Chen and Guestrin, 2016; Chen et al., 2024). The fitted model can then predict $\hat{E}(\mathbf{T}|\boldsymbol{\theta})$ for any value $\boldsymbol{\theta}$ in the domain $[0, 2.5] \times [-5, 5]^{M-1}$.

For the Metropolis-Hastings update for $\psi$, the gradient boosted trees model provides the predictions $\hat{E}\{\sum_{l \sim l'} \mathbf{I}(C_l = C_{l'})|\boldsymbol{\theta}\}$ for a given grid of $\psi$ values and fixed $\alpha_2, \ldots, \alpha_M$. Then, we can approximate the integral in (S8) by fitting a 10th-order polynomial spline to the curve of $\hat{E}\{\sum_{l \sim l'} \mathbf{I}(C_l = C_{l'})|\boldsymbol{\theta}\}$ values and integrating the polynomial. Similarly, for the Metropolis-Hastings update for each $\alpha_\eta$ with $\eta \in \{2, \ldots, M\}$, the gradient boosted trees model provides the predictions $\hat{E}\{\sum_{l=1}^{L} \mathbf{I}(C_l = \eta)|\boldsymbol{\theta}\}$ for a given grid of $\alpha_\eta$ values, other parameters being fixed. Then, we can approximate the integral in (S10) by calculating the integral of the interpolated curve of $\hat{E}\{\sum_{l=1}^{L} \mathbf{I}(C_l = \eta)|\boldsymbol{\theta}\}$ values.

Inspecting the interpolated curves for each component of $\hat{E}(\mathbf{T}|\boldsymbol{\theta})$ suggests that this procedure produces reliable estimates. While computing these estimates is initially time-consuming, we stress that they are computed a single time, outside any MCMC analysis of a particular dataset, and used for all simulated and real data analysis. After this initial procedure, evaluating (S8) and (S10) for the MCMC algorithm is very efficient.

In addition, the Metropolis-Hastings updates for $\psi$ and $\alpha_\eta$ require the sufficient quantities $\mathbf{T}$ from the corresponding MCMC draw to be valid draws from the posterior. However, to stabilize the initial draws of the spatial Potts parameters during the burn-in phase, we instead use $\mathbf{T}$ calculated from the cluster labels derived from applying $k$-means to the input

$\hat{\mathbf{\Xi}}$. After burn-in, we use $\mathbf{T}$ calculated from the cluster labels in the corresponding MCMC draw.

## 2.2 *Web Appendix B.2: Summarizing the posterior distribution*

Because the posterior distribution of the PCM is invariant to the permutation of cluster labels, there is potential for label switching. Label switching is a well-known problem in the Bayesian estimation of mixture models in which the MCMC samples simulated from the posterior distribution are non-identifiable (Papastamoulis, 2016). To ensure identifiability of parameters, we process the MCMC output via the Pivotal Reordering Algorithm (Marin, Mengersen, and Robert, 2005; Marin and Robert, 2007). For every MCMC iteration, we find the permutation $\tau \in \mathbb{N}^M$ that maximizes the element-wise product of permuted $\mu_{q\eta}$ draws $[\mu_{\cdot\tau_1}, \ldots, \mu_{\cdot\tau_M}]$ and a pivot matrix. We set the pivot matrix $[\mu^*_{\cdot\cdot}]$ to be the $[\mu_{\cdot\cdot}]$ draw that maximizes the likelihood within the burn-in phase. In particular, for each MCMC iteration $t = 1, \ldots, T$, we find the permutation $\tau^{(t)}$ that maximizes

$$[\mu^{(t)}_{\cdot\tau^{(t)}_1}, \ldots, \mu^{(t)}_{\cdot\tau^{(t)}_M}] \circ [\mu^*_{\cdot 1}, \ldots, \mu^*_{\cdot M}] = \sum_{q=1}^{Q} \sum_{\eta=1}^{M} \mu^{(t)}_{q\tau^{(t)}_\eta} \mu^*_{q\eta}. \tag{S11}$$

Then, we reorder the corresponding cluster labels $C^{(t)}_{nl}$ according to this permutation.

Having resolved the issue of label switching, the posterior mode of each cluster label, $\hat{C}_{nl}$, can be found by taking the mode of $C^{(t)}_{nl}, t = 1, \ldots, T$. To assess the uncertainty in the estimate $\hat{C}_{nl}$, the posterior probability mass function can be examined: $\hat{P}(C_{nl} = \eta) = \frac{1}{T} \sum_{t=1}^{T} \mathbf{I}(C^{(t)}_{nl} = \eta)$. The estimated cluster labels $\{\hat{C}_{nl}\}_{1 \leqslant l \leqslant L}$ can be used to segment the SPP $S_n$ (e.g., see Figure 1.2a in the main article).

Lastly, posterior inference can be conducted on the first- and second-order spatial characteristics of the clusters. The parameters $\mu_{K+1,\eta}, \ldots, \mu_{K+H,\eta}$ correspond to the cell intensities $\{\lambda_{h\eta}\}_{h=1}^{H}$ for cluster $\eta$, defined in Section 2.1 in the main article. Unscaling and uncentering the MCMC draws for these parameters would provide the posterior distribution of these

intensities. From this, the posterior means $\hat{\lambda}_{h\eta}, h = 1, \ldots, H$, can be found (see Figure 1.2b in the main article for an example of the intensity estimates $\hat{\lambda}_{h\eta}$). Similarly, the parameters $\mu_{1\eta}, \ldots, \mu_{K\eta}$ correspond to the PCF $g_\eta(\cdot)$ for cluster $\eta$, defined in Section 2.1 in the main article. Unscaling and uncentering the MCMC draws for these parameters would provide the posterior distribution of the PCF scores $\xi_{1\eta}, \ldots, \xi_{K\eta}$ for each cluster. To retrieve the PCF from the draw of scores for MCMC iteration $t$, $\left\{\xi_{1\eta}^{(t)}, \ldots, \xi_{K\eta}^{(t)}\right\}$, we first retrieve the corresponding vector of discretized function values:

$$X_\eta^{(t)} = \bar{X} + \sum_{k=1}^{K} \hat{\phi}_k \xi_{k\eta}^{(t)}, \tag{S12}$$

using the mean vector $\bar{X}$ and eigenvectors $\hat{\phi}_k$ from Equation 17 in the main article. We then square the function values and interpolate to get the corresponding PCF draw, $g_\eta(r)^{(t)}$, $r \in [\frac{R}{R_d}, R]$. Finally, the posterior mean PCF $\hat{g}_\eta(r)$ and its credible interval are calculated as the pointwise mean and pointwise credible interval of the PCF draws, respectively. See Figure 1.2c in the main article for an example of the PCF estimates $\hat{g}_\eta(r)$.

## 3. Web Appendix C: Additional simulation study details

For each SPP in a given scenario, subregions corresponding to each cluster are generated via a spatial Potts model over a $10 \times 12$ grid (where each grid region is a unit square) with $\psi$ set to 0 or 1.29. We use a function from the R package `potts` (Geyer and Johnson, 2022) to generate realizations from the spatial Potts model. The choice $\psi = 0$ corresponds to a random labelling of grid regions, whereas the choice $\psi = 1.29$ leads to more cohesive subregions. The value of 1.29 was chosen because it leads to a moderate amount of cohesion among grid regions when there are three, four, or five clusters (see Figures 1a, 1b, and 1d, respectively). In all scenarios, the $(\alpha_\eta)$ offsets are set to zero, corresponding to uniformly equal probabilities for each cluster.

[Figure 1 about here.]

Each SPP contains two cell types and is created in two stages, where unmarked points are generated first and then marked according to each cell type. We use functions from the R package `spatstat` (Baddeley, Rubak, and Turner, 2016) to generate and mark the points. In particular, local SPPs of unmarked points are generated within each subregion according to the theoretical PCF of the associated cluster, with total intensity $\lambda$. The scenarios involve the following PCFs: i) complete spatial randomness (CSR), which has the PCF $g_1(r) = 1$, ii) the Thomas process with parameters $\kappa$ and $\sigma$, which has the PCF

$$g_2(r) = 1 + \exp\{-r^2/(4\sigma^2)\}/(4\pi\kappa\sigma^2), \tag{S13}$$

and iii) the Matérn I process with parameters $\delta$ and $\kappa$, which has the PCF

$$g_3(r) = \begin{cases} 0, & r < \delta \\ \text{Undefined}, & r = \delta \\ \{\kappa/\exp(-\kappa\pi\delta^2)\}\exp\{-\kappa V(r,\delta)\}, & r > \delta, \end{cases} \tag{S14}$$

where $V(r, \delta)$ is the area of the intersection of two circles, each of radius $\delta$ with centers separated by a distance r, and $\kappa$ is selected to satisfy the equation $\lambda = \kappa \exp(-\kappa\pi\delta^2)$. The three PCFs exhibit independence, attraction, and repulsion among points, respectively; Figure 2 displays a plot of the PCFs when $\lambda = 20$. The PCF and its parameters (in the case of the Thomas or Matérn process) will vary among the clusters; Table 1 shows how the PCFs are assigned to the clusters in the three-, four-, and five-cluster scenarios.

[Figure 2 about here.]

[Table 1 about here.]

After simulating the points, points within each subregion are randomly labelled as type-1

or type-2 according to the intensity ratio of the associated cluster. The intensity of type-1 cells, $\lambda_1$, is 16 in the low intensity case and 36 in the high intensity case; the intensity of type-2 cells, $\lambda_2$, varies depending on $\lambda_1$ and the cluster (Table 1). If the cluster's intensity ratio is $1:1$, then $\lambda_1 = \lambda_2$ and there is an equal probability of a cell being labeled as type-1 or type-2. If the intensity ratio is $4:1$, then $\lambda_1 = 4\lambda_2$ and a cell is four times more likely to be labelled type-1 than type-2. Figure 1 shows example SPPs from the three-, four- and five-cluster scenarios.

## 4. Web Appendix D: Sensitivity analyses

### 4.1 *Web Appendix D.1: Resolution sensitivity analysis*

We perform sensitivity analyses with regard to the resolution of the grid and the assumed number of clusters. The first sensitivity analysis examines how the performance of the methods are affected by changing the resolution of the local estimation. We generate the SPPs on a $10 \times 12$ grid as in the main simulation study, but with four clusters, 50 subjects, $\psi = 1.29$, and intensity of type-1 cells set to 64 (the intensity of type-2 cells will depend on the intensity ratio). See Table 1 for the PCFs and intensity ratios involved in the four-cluster scenario, and Figure 1b for an example generated SPP. We use a higher intensity of cells than in the main simulation study to ensure that there is at least 20 cells per grid region when the fine resolution is used. The methods are fitted on this data under three resolutions: the coarse resolution with a $5 \times 6$ grid, the middle resolution with a $10 \times 12$ grid (the true resolution), and the fine resolution with a $20 \times 24$ grid (Figure 3). Given a grid, the input $\hat{\boldsymbol{\Xi}}$ is computed from the generated data as described in Section 3 in the main article and then passed to the methods.

[Figure 3 about here.]

To enable comparison between models fitted under different resolutions, the estimated clus-

ter labels from the middle and coarse resolution models are converted to the fine resolution. That is, the $20 \times 24$ grid is superimposed upon the estimated cluster labels, and each grid region of the finer grid shares the same cluster label as the grid region that it overlaps. The dimensions of the middle and coarse grids have been chosen such that the finer grid regions do not cross the boundaries of the coarser grid regions. The true cluster labels, which were generated on a $10 \times 12$ grid, are also converted to the fine resolution in this way. Then, the clusterings proposed by the models can be compared to the true clustering through the ARI.

As shown in Figure 4, for all three resolutions, the PCM outperforms the competing algorithms. Both the PCM and non-spatial PCM are generally the best at the true resolution ($10 \times 12$), but perform about the same at the coarse resolution ($5 \times 6$) as compared to the true resolution. Therefore, it appears to be better to underestimate the resolution than to overestimate it.

[Figure 4 about here.]

## 4.2 *Web Appendix D.2: Number of Clusters sensitivity analysis*

The second sensitivity analysis examines how well the PCM can perform when the assumed number of clusters is different from the truth. We use the three-cluster and five-cluster scenario as in the main simulation study, with $N = 50, \psi = 1.29$, and low total intensity $\lambda$. We measure the performance of the PCM when it is set to the true number of clusters (three and five, respectively) or a different number of clusters. Specifically, for both the three- and five-cluster scenario, we fit the PCM for the numbers of clusters $M \in \{2, \dots, 8\}$.

For the three-cluster scenario, the best performance in terms of the ARI is achieved at the true number of clusters, $M = 3$ (Figure 5a). The performance decreases slightly as the number of clusters increases, before plateauing at approximately 0.75. For the five-cluster scenario, the best performance is achieved at $M = 6$ clusters (Figure 5b). The performance

at higher numbers of clusters, $M = 7$ and $M = 8$, is virtually the same. It is generally better to have too many clusters, rather than too few.

[Figure 5 about here.]

We also measure the computation time across the different numbers of clusters (Figure 6). For either the three- or five-cluster scenario, the computation time increases exponentially as $M$ increases. For $M = 6$ clusters or below, the computation time is less than an hour; for more clusters, the computation time can be as long as 5 hours on average.

[Figure 6 about here.]

## 5. Web Appendix E: Description of the motivating dataset

The dataset that motivates this work is a set of SPPs obtained from multiplex immunofluorescence (mIF) images of diseased pancreatic tissue. The mIF images were obtained from patients at the University of Michigan Pancreatic Cancer Clinic who had undergone surgical resection for various pancreatic diseases. The study was done in accordance with the University of Michigan Institutional Review Board approval. Of these patients, 71 were diagnosed with pancreatic ductal adenocarcinoma (which we refer to as the cancerous disease group) and 34 were diagnosed with chronic pancreatitis (which we refer to as the non-cancerous disease group). Images from patients in other pancreatic disease groups were obtained (see Krishnan et al. (2022)), but we focus on the two aforementioned disease groups for the demonstration of our method. Multiple images were collected for some patients, but we simplify the analysis by randomly selecting one image for each patient, for a total of 105 images.

As mentioned in Section 1 in the main article, multiplex imaging like mIF allows for simultaneous detection of multiple phenotype markers on a single tissue section (Tan et al., 2020). The mIF images were analyzed by the inForm software (PerkinElmer, 2012) to locate

cell centroids and determine cell types. The centroids and the types of the cells make up the SPP corresponding to each mIF image. Figure 7 shows six example SPPs obtained from the mIF images. There are six known cell types present in the data, namely, epithelial, helper T, CTL, APC, Treg, and PD-L1$^+$ CD8$^+$, which are all part of the immune system (Spiering, 2015). The PD-L1$^+$ CD8$^+$ cell type refers to immune cells with the phenotype markers PD-L1$^+$ and CD8$^+$. The epithelial and immune cell types play important roles in the development of pancreatic cancer. The mIF images also contain cells of unknown type, i.e., they may have one of the six cell types mentioned or some other type. Such cells have been classified as "other".

[Figure 7 about here.]

About 5.63% of cells have the same spatial coordinates as another cell. For such spatial coordinates, we retain the most prevalent cell type that is not "other" and omit the rest. If there are no known cell types at a coordinate, the "other" type is retained. After doing this, the cell types from most prevalent to least prevalent across subjects (average intensity, standard deviation in number of points per 10,000 microns$^2$) are other (35.78, 28.18), epithelial (27.91, 24.79), helper T (5.35, 7.17), CTL (4.33, 11.79), APC (2.37, 2.61), Treg (1.11, 7.67), and PD-L1$^+$ CD8$^+$ (0.78, 1.98).

The sampling window of the SPP retrieved from each mIF image, as determined by the minimum and maximum x- and y- coordinates of the cells, varies by subject. The average (standard deviation) dimensions of the window are 671.77 microns (36.26) by 504.79 microns (5.01). Then, the average (standard deviation) intensity of all cells combined is 77.63 (34.60) points per 10,000 micron$^2$ across images.

## 6. Web Appendix F: Clustering proportions for the analysis of mIF images

[Table 2 about here.]

## References

Baddeley, A., Rubak, E., and Turner, R. (2016). *Spatial Point Patterns : Methodology and Applications with R.* CRC Press.

Casella, G. and Berger, R. L. (2002). *Statistical Inference.* Duxbury Press, Pacific Grove, 2nd edition.

Chen, T. and Guestrin, C. (2016). XGBoost: A scalable tree boosting system. In *Proceedings of the 22nd ACM SIGKDD International Conference on Knowledge Discovery and Data Mining*, KDD '16, pages 785–794, New York, NY, USA. Association for Computing Machinery.

Chen, T., He, T., Benesty, M., Khotilovich, V., Tang, Y., Cho, H., Chen, K., Mitchell, R., Cano, I., Zhou, T., Li, M., Xie, J., Lin, M., Geng, Y., Li, Y., Yuan, J., and implementation), X. c. b. X. (2024). XGBoost: eXtreme Gradient Boosting.

Chib, S. and Greenberg, E. (1995). Understanding the metropolis-hastings algorithm. *The American Statistician* **49,** 327–335. Publisher: [American Statistical Association, Taylor & Francis, Ltd.].

Geyer, C. J. and Johnson, L. (2022). potts: Markov Chain Monte Carlo for Potts models. manual.

Krishnan, S. N., Mohammed, S., Frankel, T. L., and Rao, A. (2022). GaWRDenMap: A quantitative framework to study the local variation in cell–cell interactions in pancreatic disease subtypes. *Scientific Reports* **12,** 3708. Publisher: Nature Publishing Group.

Marin, J., Mengersen, K., and Robert, C. (2005). Bayesian modelling and inference on mixtures of distributions. In *Handbook of Statistics*, volume 25, pages 577–590.

Marin, J. and Robert, C. (2007). *Bayesian Core: A Practical Approach to Computational Bayesian Statistics.* Springer-Verlag.

Papastamoulis, P. (2016). label.switching: An R package for dealing with the label switching

problem in MCMC outputs. *Journal of Statistical Software, Code Snippets* **69,** 1–24.

PerkinElmer (2012). *inForm Advanced Image Analysis Software – For Accurately Quantifying Biomarkers in Tissue Sections.*

R Core Team (2021). R: A language and environment for statistical computing. manual, R Foundation for Statistical Computing, Vienna, Austria.

Reich, B. J. and Gardner, B. (2014). A spatial capture-recapture model for territorial species. *Environmetrics* **25,** 630–637.

Reich, B. J. and Ghosh, S. K. (2019). *Bayesian Statistical Methods.* CRC Press, Boca Raton, FL.

Spiering, M. J. (2015). Primer on the immune system. *Alcohol research: current reviews* **37,** 171. Publisher: National Institute on Alcohol Abuse and Alcoholism.

Tan, W. C. C., Nerurkar, S. N., Cai, H. Y., Ng, H. H. M., Wu, D., Wee, Y. T. F., Lim, J. C. T., Yeong, J., and Lim, T. K. H. (2020). Overview of multiplex immunohistochemistry/immunofluorescence techniques in the era of cancer immunotherapy. *Cancer Communications* **40,** 135–153. Publisher: Wiley Online Library.

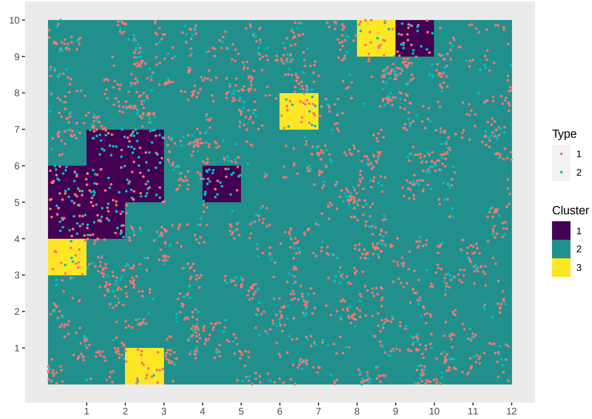


(a) $M = 3, \psi = 1.29, \lambda_1 = 16$

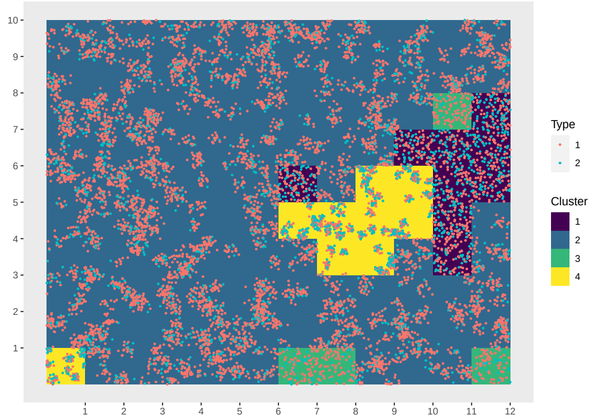


(b) $M = 4, \psi = 1.29, \lambda_1 = 64$

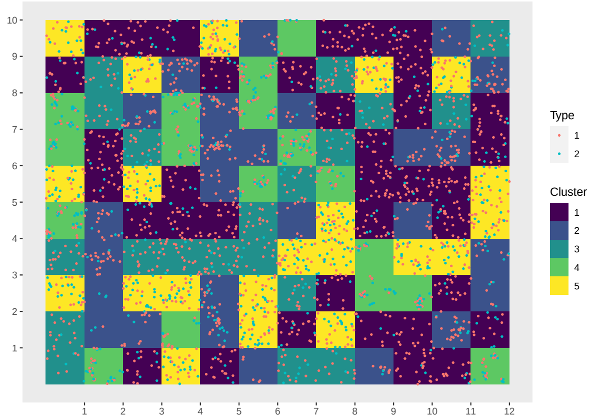


(c) $M = 5, \psi = 0, \lambda_1 = 16$

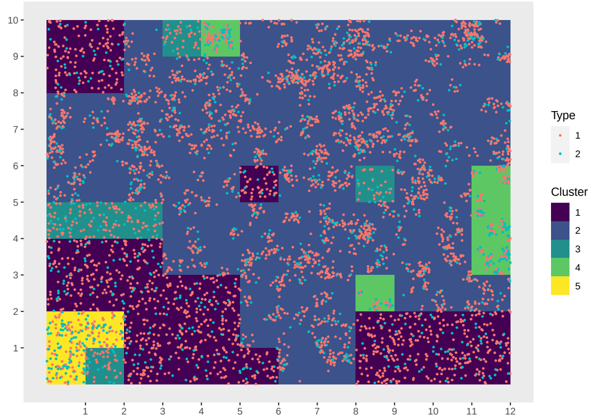


(d) $M = 5, \psi = 1.29, \lambda_1 = 36$

**Figure 1**: Example generated SPPs for the simulation study. Only the intensity of type-1 cells is indicated; the intensity of type-2 cells depends on the intensity ratio. (a) Example SPP for the scenario with three clusters, $\psi = 1.29$, and intensity of type-1 cells set to 16. (b) Example SPP for the scenario with four clusters, $\psi = 1.29$, and intensity of type-1 cells set to 64. (c) Example SPP for the scenario with five clusters, $\psi = 0$, and intensity of type-1 cells set to 16. (d) Example SPP for the scenario with five clusters, $\psi = 1.29$, and intensity of type-1 cells set to 36.

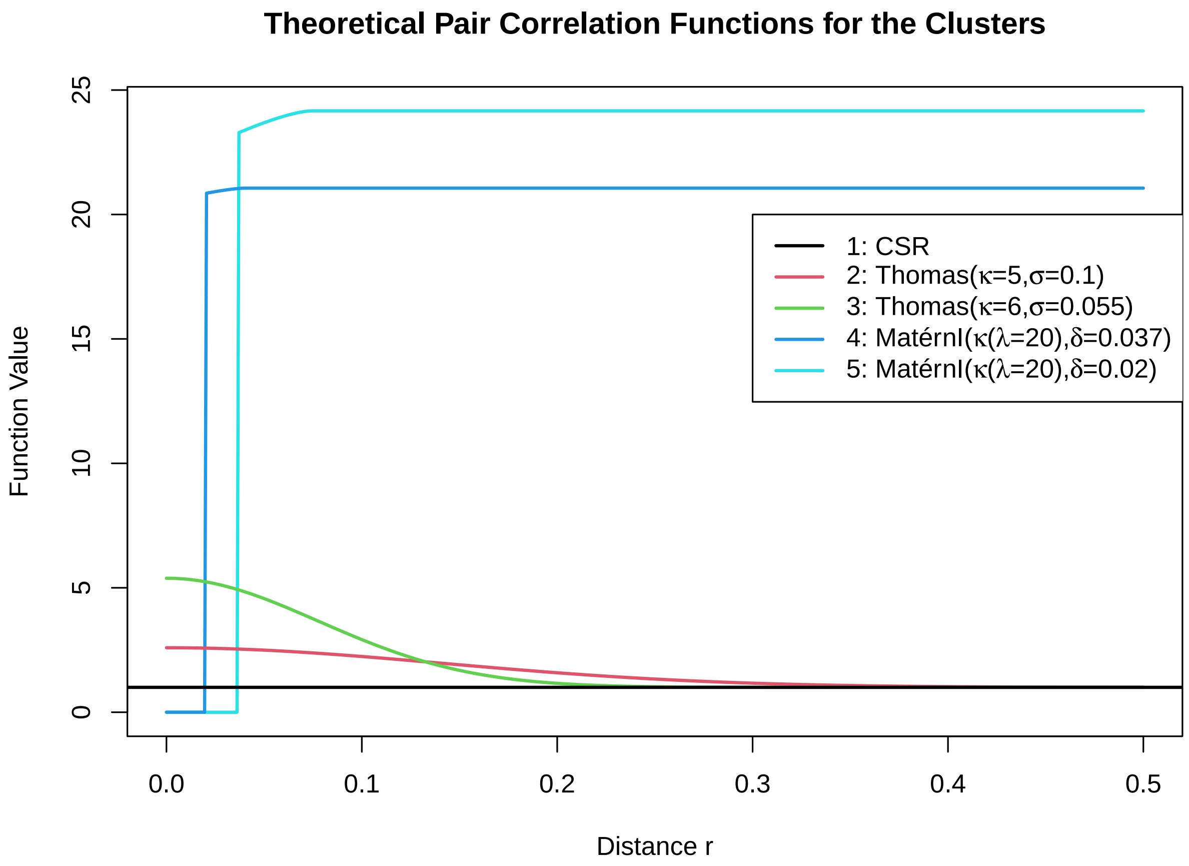


**Figure 2**: Theoretical PCFs used in the simulation study and sensitivity analysis.

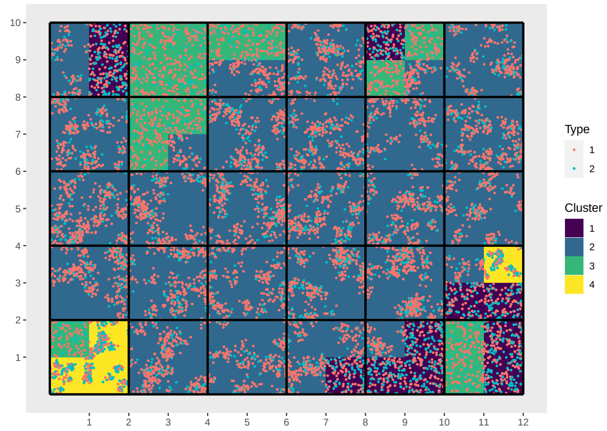


(a) Coarse Resolution: $5 \times 6$

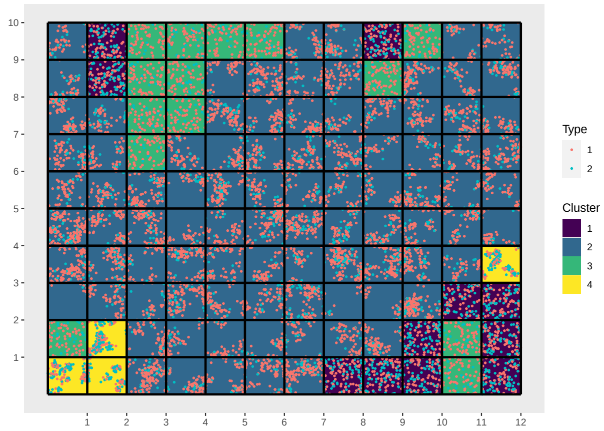


(b) Middle Resolution: $10 \times 12$

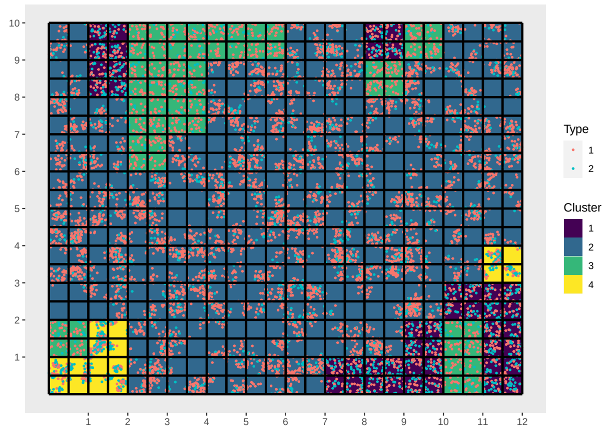


(c) Fine Resolution: $20 \times 24$

**Figure 3**: The three resolutions (coarse, middle, and fine) in the sensitivity analysis, shown as black grids overlaid on the same SPP. The SPP was generated at the middle resolution with the settings $M = 4, \psi = 1.29$, and $\lambda_1 = 64$ ($\lambda_2$ will depend on the intensity ratio).

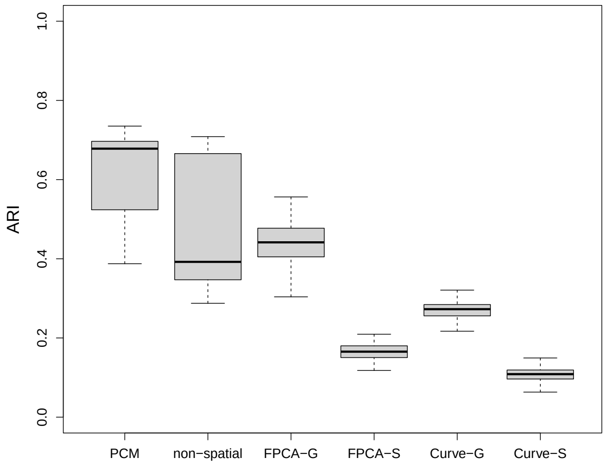


(a) Coarse Resolution

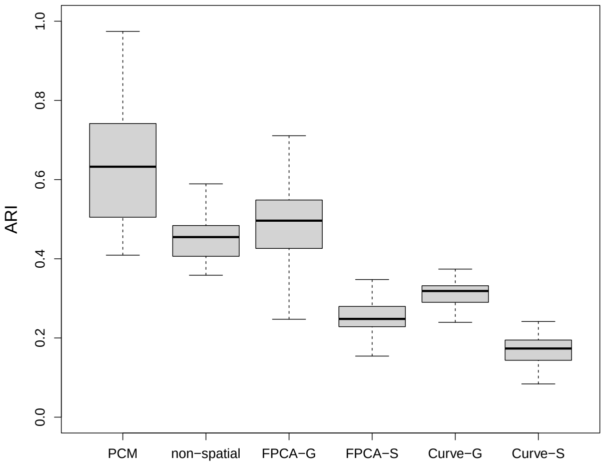


(b) Middle Resolution

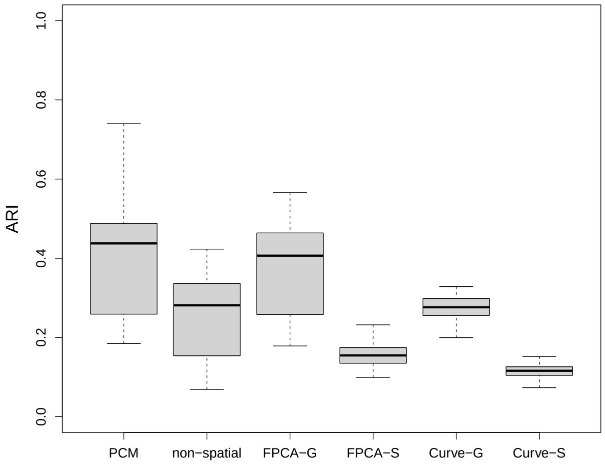


(c) Fine Resolution

**Figure 4**: Results for the resolution sensitivity analysis. ARI is the adjusted Rand index. Our proposed algorithm is denoted as PCM, whereas the non-spatial PCM is denoted as ‘non-spatial’. FPCA-G, FPCA-S, Curve-G, and Curve-S are four variations of the $k$-means algorithm.

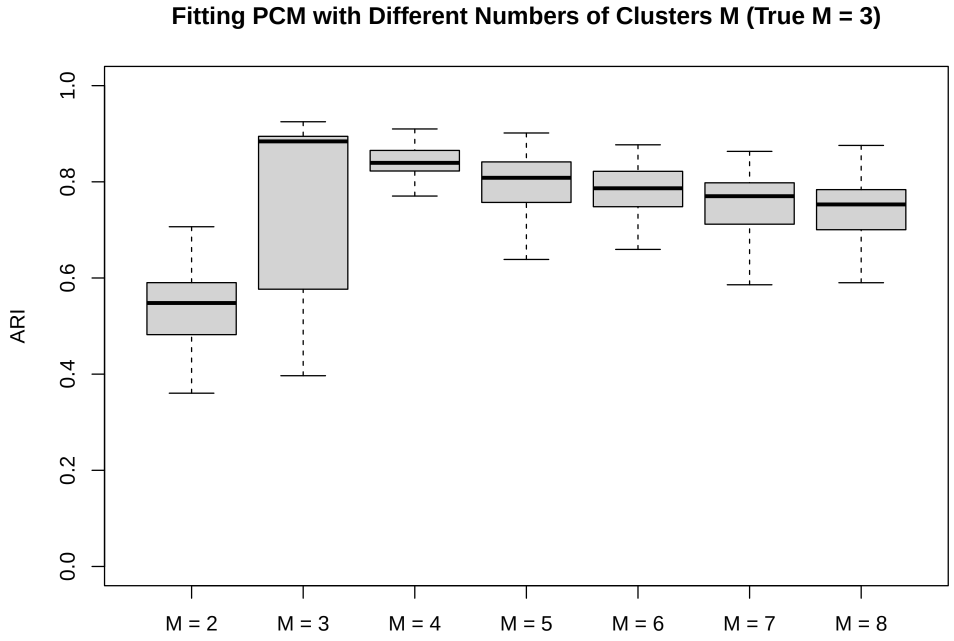


(a)

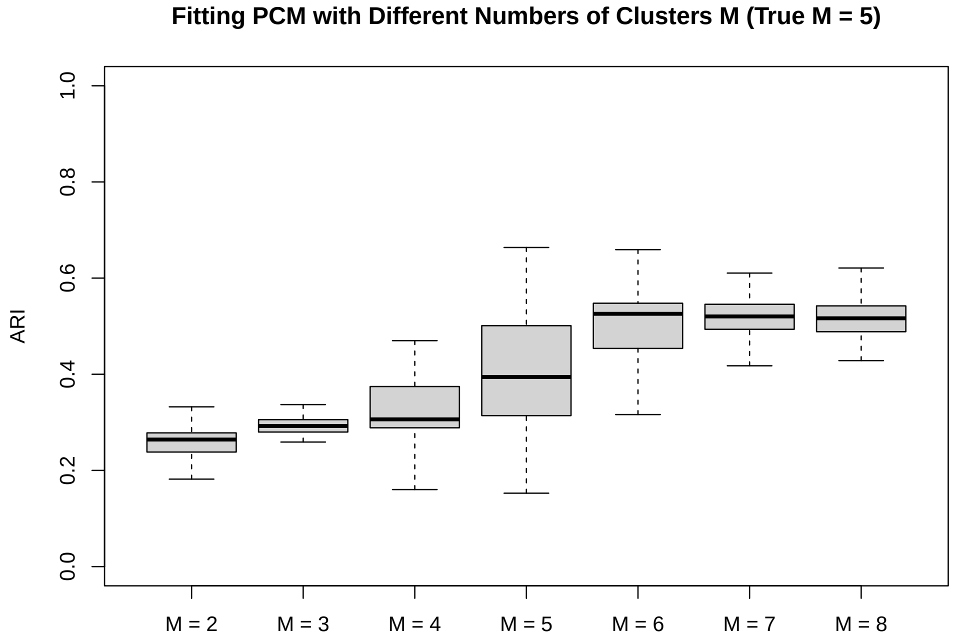


(b)

**Figure 5**: Results for the number of clusters sensitivity analysis. For both the three- and five-cluster scenario, the PCM is fitted for $M = 2, \ldots, 8$ clusters. ARI is the adjusted Rand index. (a) The performance of the PCM when data is generated according to the three-cluster scenario. (b) The performance of the PCM when data is generated according to the five-cluster scenario.

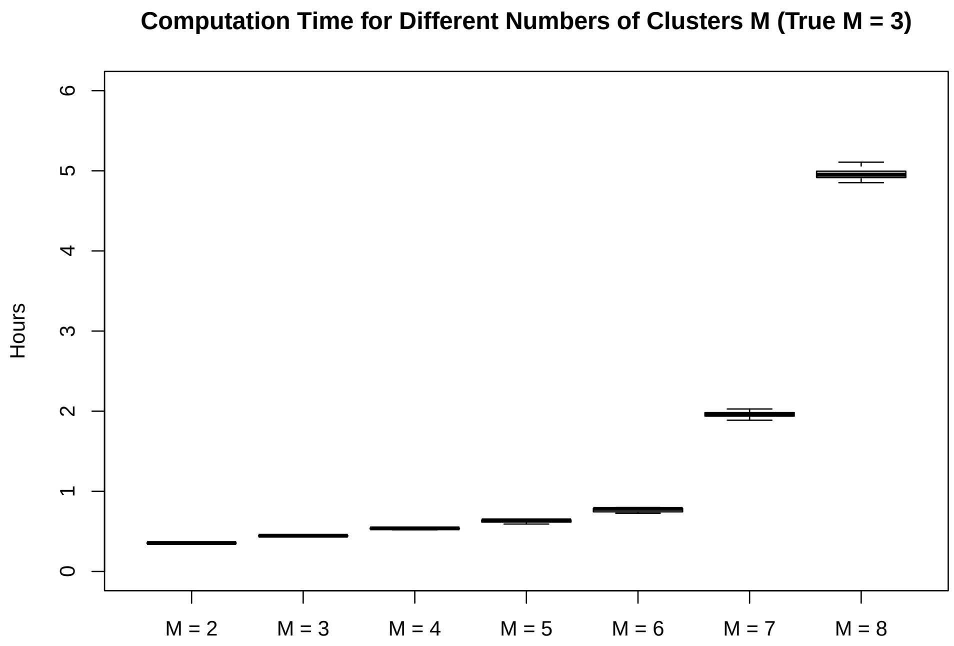


(a)

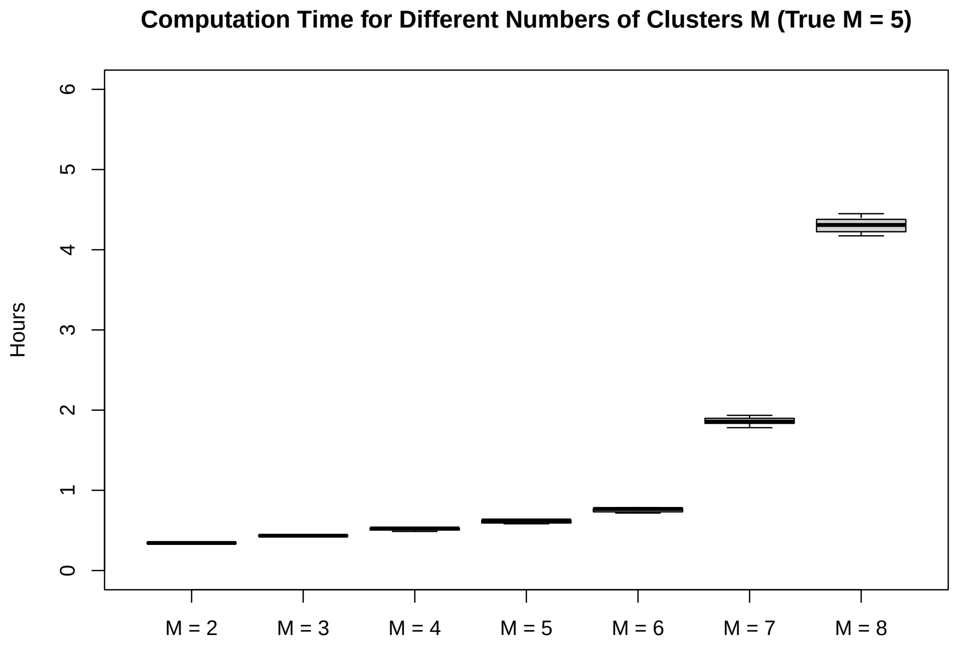


(b)

**Figure 6**: Computation times for the number of clusters sensitivity analysis. For both the three- and five-cluster scenario, the PCM is fitted for $M = 2, \dots, 8$ clusters. (a) The computation time of the PCM when data is generated according to the three-cluster scenario. (b) The computation time of the PCM when data is generated according to the five-cluster scenario.

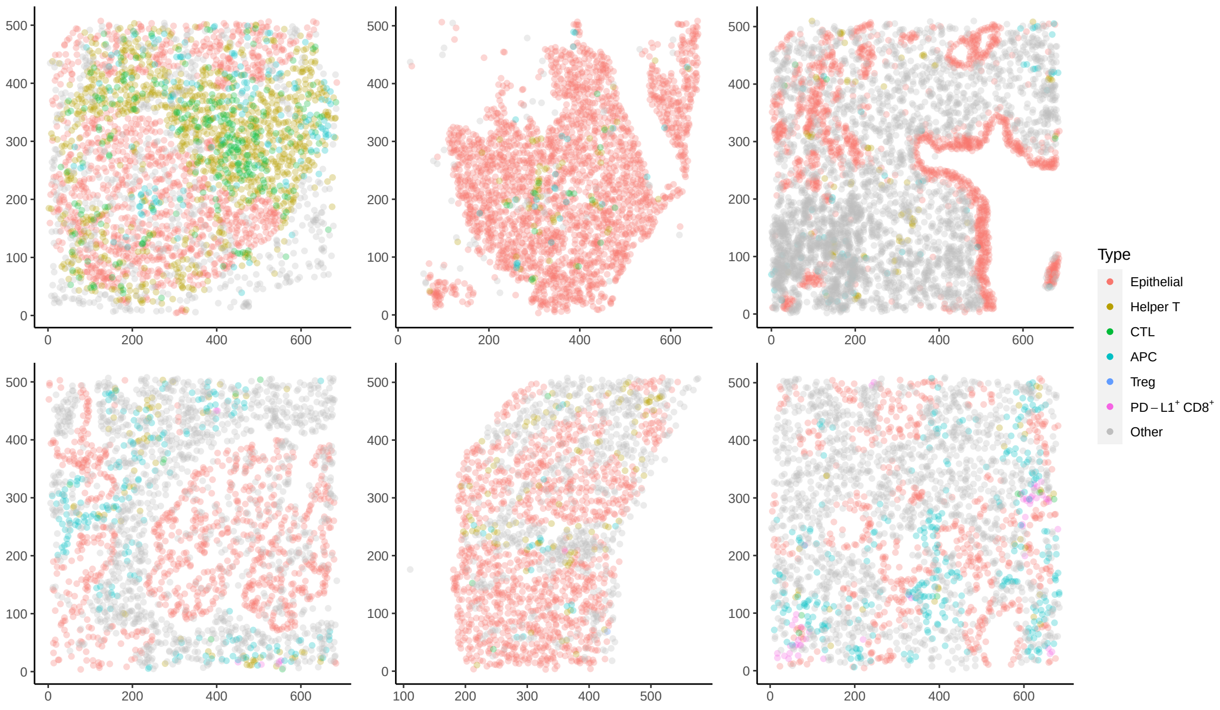


**Figure 7**: Six representative SPPs obtained from mIF images of pancreatic tissue. Points representing cell centroids are colored according to six cell types, as well as other (see legend). The top row shows three SPPs from the non-cancerous disease group and the bottom row shows three SPPs from the cancerous disease group.

Table 1: PCF and intensity ratio for each cluster, for the three-, four-, and five-cluster scenarios.

| Scenario | Cluster | PCF | Intensity Ratio ($\lambda_1 : \lambda_2$) |
|---|---|---|---|
| Three Clusters | 1 | CSR | 1:1 |
| | 2 | Thomas($\kappa = 5, \sigma = 0.1$) | 4:1 |
| | 3 | MatérnI($\kappa(\lambda), \delta = 0.037$) | 4:1 |
| Four Clusters | 1 | CSR | 1:1 |
| | 2 | Thomas($\kappa = 5, \sigma = 0.1$) | 4:1 |
| | 3 | MatérnI($\kappa(\lambda), \delta = 0.037$) | 4:1 |
| | 4 | Thomas($\kappa = 6, \sigma = 0.055$) | 1:1 |
| Five Clusters | 1 | CSR | 4:1 |
| | 2 | Thomas($\kappa = 5, \sigma = 0.1$) | 4:1 |
| | 3 | MatérnI($\kappa(\lambda), \delta = 0.037$) | 4:1 |
| | 4 | Thomas($\kappa = 6, \sigma = 0.055$) | 1:1 |
| | 5 | MatérnI($\kappa(\lambda), \delta = 0.02$) | 1:1 |

Table 2: Cluster proportions (%). The proportions are calculated as the number of grid regions belonging to a given cluster divided by the total number of grid regions in the group. Each subject has 130 grid regions; the non-cancerous disease group has 34 subjects and 4420 grid regions, and the cancerous disease group has 71 subjects and 9230 grid regions.

| Cluster | 1 | 2 | 3 | 4 | 5 | 6 | 7 | 8 |
|---|---|---|---|---|---|---|---|---|
| Non-Cancerous Disease Group | 0.3 | 41.1 | 1.1 | 47.4 | 6.1 | 1.5 | 2.5 | 0.0 |
| Cancerous Disease Group | 3.7 | 67.5 | 1.2 | 8.2 | 6.6 | 5.0 | 6.5 | 1.3 |
